# Supplementary material for: Ultra-miniaturized Bloch mode metasplitters for one-dimensional grating waveguides
Source: arXiv:2410.14531 source file (2024-10-18)
Supplement: Supplementary file 1 [file AOSakin_supp_metasplitter.pdf]

# Supplemental information: Ultra-miniaturized Bloch mode metasplitters for one-dimensional grating waveguides

Ahmet Oguz Sakin[1], Hamza Kurt[2], Mehmet Unlu[1*]
[1]Department of Electrical and Electronics Engineering, TOBB University of Economics and Technology, Ankara, Turkey
[2]School of Electrical Engineering, Korea Advanced Institute of Science and Technology (KAIST), Daejeon, Republic of Korea
***Corresponding author:** munlu@etu.edu.tr

In this supplementary document, we begin with the design of one-dimensional grating waveguide (1DGW) topologies tailored for true time delay applications in the L-band. Following this, we derive analytical expressions that establish a correlation between the peak value of the time-domain Poynting vector, dispersion, and pulse broadening, facilitating the design of structures with optimal dispersion profiles and broadband characteristics. A thorough analysis of the electric field distribution across all structures is then provided. Lastly, we demonstrate the consistency between simulation and measurement results, tolerating the observed band shift between them.

## S1 Design of one-dimensional grating waveguides for L-band applications

Figure S1 presents the key design criteria for the one-dimensional grating waveguide (1DGW) topology utilized in this study. The appropriate structural parameters of the 1DGW for L-band applications are determined by the product of the normalized peak power level, denoted as $A_n$, and the normalized true time delay, represented as $D_n$, for the 50-period structure. As illustrated in Figure S1-(a), the parameters are selected to facilitate the evaluation of metasplitter structures' performance in topologies near both optimized and non-optimized regions, based on time delay and peak power characteristics. Therefore, the corrugation width $(w_d)$ is set to 2.1 $\mu$m, and the grating period $(\lambda)$ is set to 380 nm, with a $50\%$ duty cycle. To generate this optimization, an ultrashort Gaussian signal with a width of 90 fs at 1580 nm is used as input to the system. The strip waveguide width $(w_s)$ connecting the 1DGW to the grating coupler is chosen to support 2 TE and 2 TM modes, allowing for the evaluation of any potential mode conversion after the metasplitter devices. However, no such mode conversion was observed, owing to the superior mode protection provided by the meta devices. The inner waveguide width $(w_c)$ is chosen as 450 nm to support an average level of dispersion, considering the width contrast with the strip waveguide width $(w_s)$. The band diagram shown in Figure S1-(b) is calculated using the 3D plane wave expansion method, based on the optimized design parameters. As shown in Figure S1-(c), the relatively flat slope of band 3 corresponds to a low group velocity region. The group velocity, $v_g$, is expressed as $v_g = \frac{d\omega}{dk}$, where $\omega$ represents the angular frequency and $k$ denotes the wave vector. In this region, the derivative $\frac{d\omega}{dk}$ is small, resulting in a low group velocity, a key characteristic of slow light. This slow light effect, coupled with the broad wavelength range over which it is sustained, makes band 3 highly suitable for true-time delay applications. The corresponding group index values are presented in Figure S1-(d). The group index $n_g$ is determined to be 6.2 at 1580 nm, approximately $48\%$ higher than that of a standard strip waveguide. This value increases to 12.58 at 1603 nm, clearly highlighting the significant design constraints associated with the wavelength-selective broadband nature of the metasplitter.

## S2 Figure of merit formula for time-domain heuristic design with broadband and dispersion awareness

In the metasplitter design, the figure of merit of the time-domain heuristic algorithm is defined by the peak intensity of the time-domain Poynting vector at the output. This choice ensures that the design simultaneously

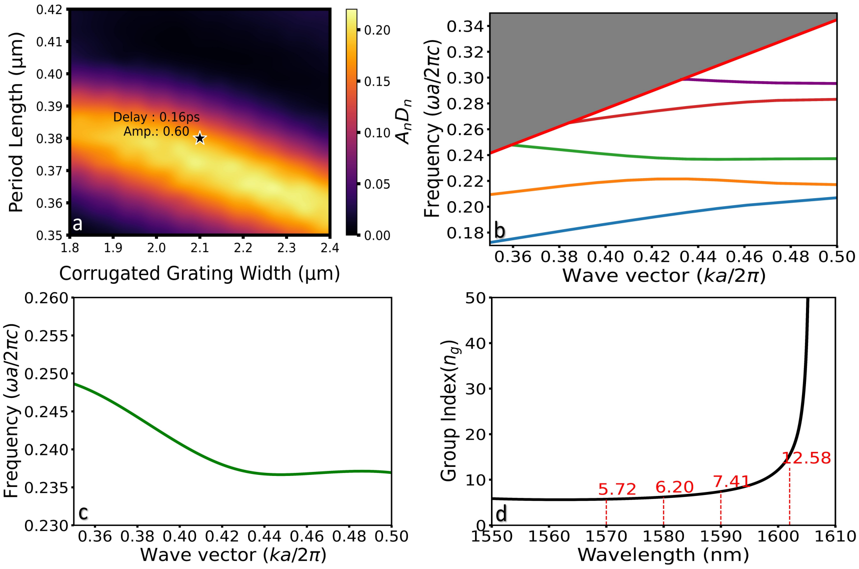


**Supplementary Figure 1:** (a) Design parameter space illustrating the relationship between the period length and the corrugated grating width, based on the product of normalized peak power and normalized time delay. (b) Band structure of the designed 1DGW. (c) Dispersion relation showing the frequency behavior of the selected mode. (d) Group index variation with respect to wavelength.

optimizes the wavelength-selective dispersion profile and broadband requirements without additional steps. Also, a Gaussian signal with a 90 fs pulse duration at 1580 nm is used to cover the targeted ultra-wideband range in the inverse design process. To demonstrate the appropriateness of the figure of merit, the Poynting vector output signal, after propagating through the dispersive medium of the 1DGW, is expressed in Equation S1.

$$S(t,z) = \frac{E_0^2}{\eta(z)} \exp\left(-\frac{t^2}{\tau(z)^2}\right) \cos^2(\omega_0 t + \phi(t,z)) \tag{S1}$$

Here, $\tau(z)$ represents the broadened pulse duration at a distance $z$, $\omega_0$ is the central angular frequency of the pulse, and $\phi(t,z)$ denotes the phase shift introduced by the dispersion. $E_0$ is the peak amplitude of the electric field, and $\eta(z) = \frac{\eta_0}{n(z)}$ represents the impedance of the medium, where $\eta_0$ is the intrinsic impedance of free space and $n(z)$ is the refractive index of the dispersive structure. The Gaussian pulse is typically symmetric in time, with the peak value of the time-domain Poynting vector occurring at the center of the pulse, at $t = 0$. As the pulse propagates through a dispersive medium, the pulse duration $\tau(z)$ increases due to broadening, which directly influences the peak value of the time-domain Poynting vector, $S_{\text{peak}}(z)$, since the energy is spread over a longer time frame. The derivation of the peak value of the time-domain Poynting vector is provided in Equation S2.

$$S_{\text{peak}}(z) \propto \frac{S_0}{\tau_0 \sqrt{1 + \left(\frac{z}{L_D}\right)^2}} \tag{S2}$$

Here, $\tau_0$ is the initial pulse duration, $L_D = \frac{\tau_0^2}{|\beta_2|}$ is the dispersion length, $\beta_2$ is the second-order dispersion coefficient, and $S_0$ is the peak value of the time-domain Poynting vector at $t = 0$. As demonstrated in Equation S2, the peak value of the time-domain Poynting vector is directly affected by both pulse broadening and the dispersion properties of the structure. Consequently, optimizing the peak value of the time-domain Poynting vector inherently involves achieving optimal dispersion and broadband characteristics.

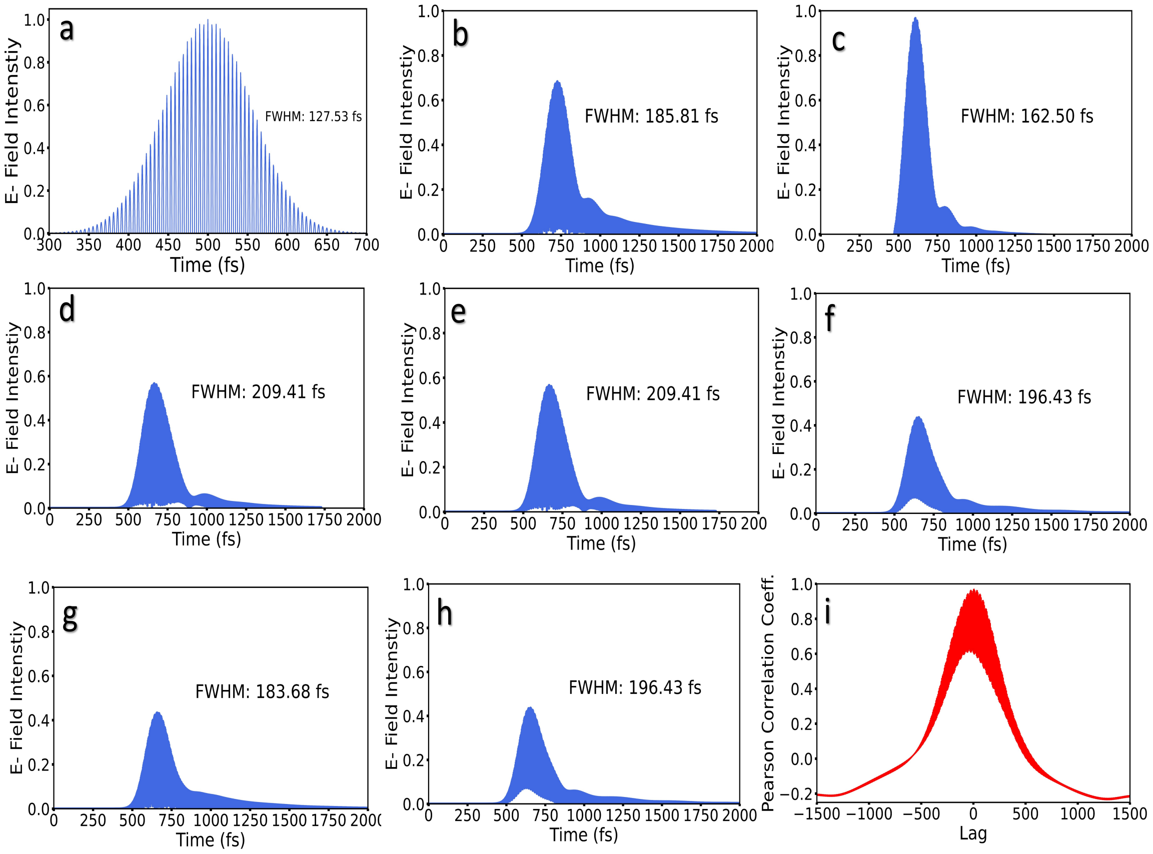


**Supplementary Figure 2:** (a) Gaussian input signal. (b) Output from a 1DGW with 16 periods. (c) Corresponding output from half of the 16-period 1DGW structure. (d, e) Outputs for the 1x2 metasplitter structure. (f-h) Outputs for the 1x3 metasplitter structure: (f, h) symmetrical channels, (g) straight channel. (i) Pearson correlation coefficient calculation between symmetrical and straight channel outputs at different lag levels.

Due to the correlation between the E-field and the Poynting vector, as shown in Equation S1, the peak value of the time-domain Poynting vector is calculated using the E-field signal outputs. The corresponding E-field results are shown in Figure S2. Figure S2-(a) illustrates the Gaussian input signal employed in the heuristic optimization of the metastructures. Typically, each channel in the metasplitter structures consists of 16 periods of the 1DGW from input to output. Figure S2-(b) shows the output of the ultrashort pulse signal from a 1DGW with 16 periods, where the peak E-field intensity is approximately 0.63, resulting in a peak power intensity of about 0.4, as the peak power intensity is proportional to the square of the peak E-field intensity. The power monitors in the 3D Finite-Difference Time-Domain (FDTD) simulations, used to characterize the time-domain response of metasplitter designs, are placed at the tip of the meta structures, covering only

half of the 16-period 1DGW. Therefore, the analysis should also include the half-system of the 16-period 1DGW, as illustrated in Figure S2-(c). In this configuration, the peak E-field intensity reaches approximately 0.98, corresponding to the peak power intensity of 0.96. Figure S2-(d) and (e) depict the outputs for the 1x2 metasplitter structure, which shows symmetry in both channels, resulting in identical outputs. The peak E-field intensity is approximately 0.57, resulting in the peak power intensity of 0.65 across the two channels, with a Full Width at Half Maximum (FWHM) expansion of 47 fs compared to the half-system of the 1DGW. Figure S2-(f) to (h) illustrate the outputs for the 1x3 metasplitter structure: (f) and (h) show the symmetrical channels, while (g) displays the straight channel. The average peak power intensity is 0.56, with FWHM expansions of 33 fs for the symmetrical ports and 20 fs for the straight channel. Moreover, to assess the similarity between the symmetrical and straight channel outputs, the Pearson correlation coefficient is calculated. As shown in Figure S2-(i), a value very close to 1 is obtained at lag 0, indicating a high degree of similarity. As a result of the examined scenarios, it is evident that the deviation ratio remains notably low despite using an ultra-miniature structure. This preservation of peak intensity enables the design of a meta-structure with low loss, uniform characteristics, and broadband frequency response, as stated in the main text.

## S3 Electric field mode distributions

Figure S3-(a) to (o) presents the E-field mode distributions for both the 1DGW and the designed metastructures. Figure S3-(a) to (c) shows the results at 1580 nm. For the 1x2 splitter, Figure S3-(d) to (i) illustrates the field distributions, and for the 1x3 metasplitters, Figure S3-(j) to (o) details the distributions within the 1550-1600 nm range for both structures.

## S4 Analysis of band shift between simulations and measurements

As outlined in the main text, the 1DGW structure exhibits significant sensitivity to dimensional variations, such as sidewall roughness, period, and corrugation width. Fabrication imperfections cause shifts in the band structure due to alterations in these parameters. Additionally, the small pixel size of 100 nm introduces fabrication imperfections, such as rounded corners in metastructures, which further affect the uniformity ratio between channels in metasplitter designs. When comparing the 1 dB bandwidths of the measurement and simulation results presented in the main text, the average shift is found to be 26 nm for the 1DGW, 13 nm for the 1x2 metasplitter, and 9 nm for the 1x3 metasplitter, resulting in an overall average shift of 16 nm. The band narrowing is disregarded due to its minimal impact, as it is calculated to be only 1 nm between the simulated and measured results for the 1DGW structure. As shown in Figure 4S-(a) to (c), when the measurement results are shifted by 16 nm, the 1DGW, 1x2, and 1x3 metasplitters respectively demonstrate that the measurement and simulation results are in good agreement.

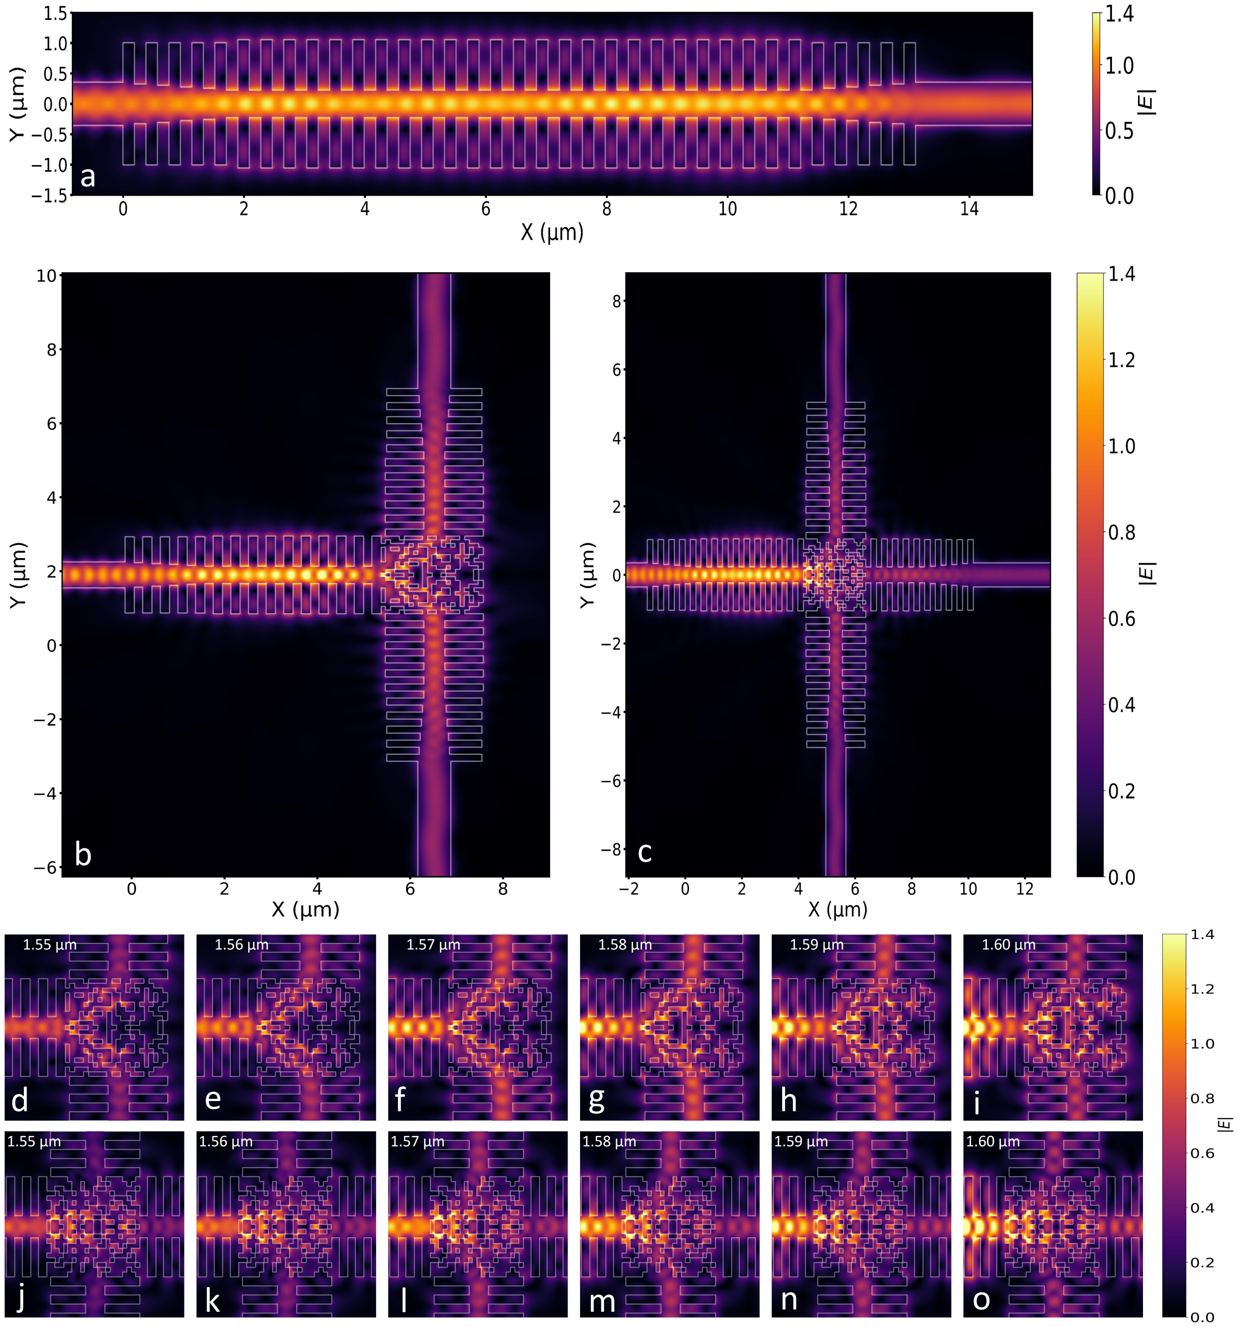


**Supplementary Figure 3:** (a-c) E-field mode distributions for the 1DGW and designed 1x2 and 1x3 metastructures at 1580 nm, respectively. (d-i) E-field distributions for the 1x2 metasplitter across the 1550-1600 nm range. (j-o) E-field distributions for the 1x3 metasplitter within the same wavelength range.

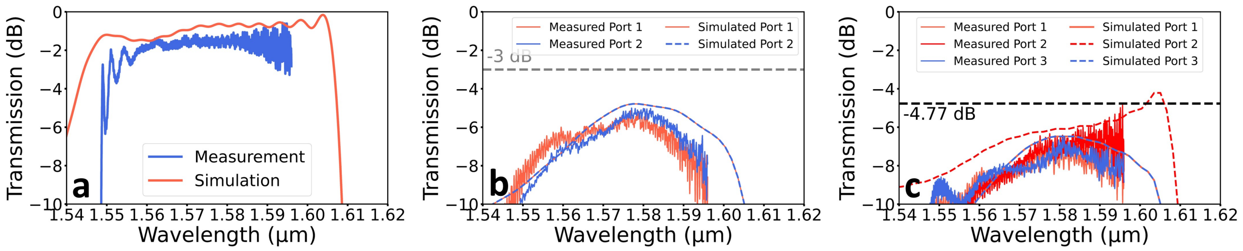


**Supplementary Figure 4:** Comparison of measured and simulated transmission after applying a 16 nm shift to the measured data. (a) for the 1DGW, (b) for the 1x2 metasplitter, and (c) for the 1x3 metasplitter.
